# Supplementary material for: Deep Policy Gradient Methods Without Batch Updates, Target Networks, or Replay Buffers
Source: arXiv:2411.15370 source file (2025-05-21)
Supplement: Supplementary file 1 [file additional_ablations.tex]

\clearpage
\newpage

%%%%%%%%%%%%%%%%%%%%%%%%%%%%%%%%%%%%%%%%%%%%%%%%%%%%%%%%%%%%
\section{Additional Ablations on Simple Environments}

\begin{wrapfigure}{r}{0.6\textwidth}
\begin{minipage}{0.59\textwidth}
\vspace{-0.5cm}
\centering
\begin{subfigure}{.3\textwidth}
    \includegraphics[width=\columnwidth]{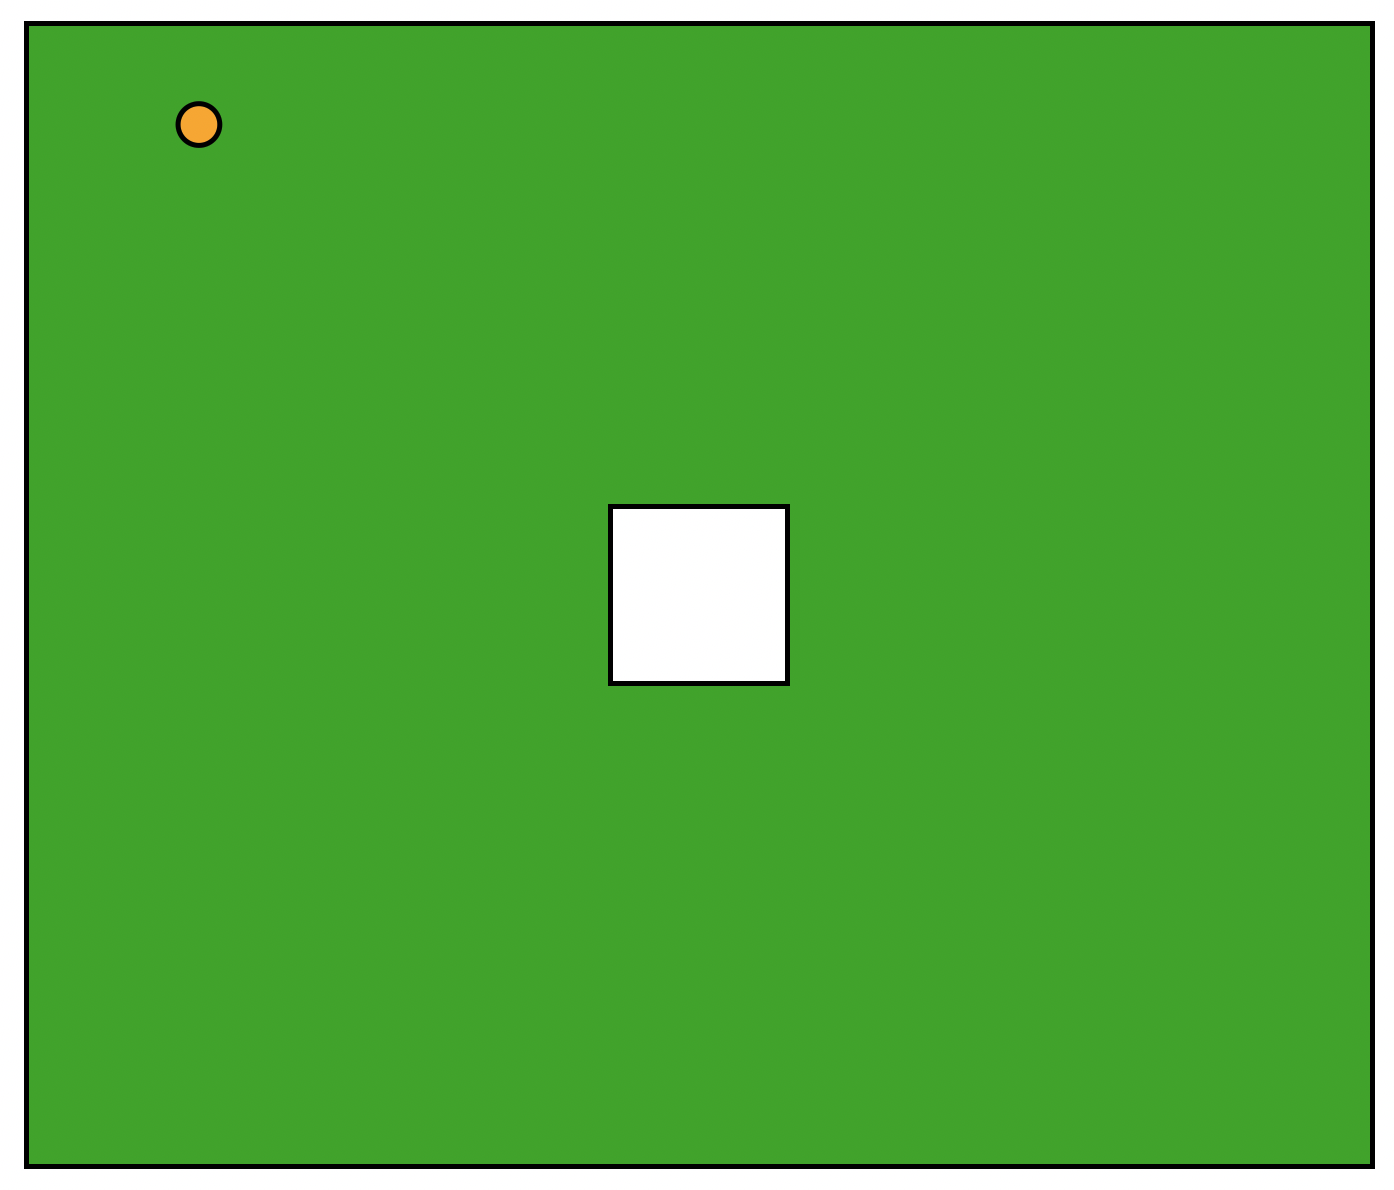}
\end{subfigure}
\caption{The Dot Reacher Task}
\label{fig:dot_reacher}

\begin{algorithm}[H]
    \caption{AVG + Distribution Entropy}
    \label{algo:avg_dist}
    \begin{spacing}{1.25}        
    \begin{algorithmic}
        \STATE {\bfseries Initialize}  $\theta$, $\phi$, $\gamma$, $\eta$, $\alpha_{\pi}$, $\alpha_Q$ \\
        \FOR{however many episodes}
            \STATE Initial S (first state of the episode)
            \WHILE{S is not terminal}
                \STATE $A_{\theta} = f_\theta (\epsilon; S) \text{ where } \epsilon \sim \mathcal{N}(0,1) $ \\
                \STATE Take action $A$, observe $S', R$ \\
                \STATE Update \emph{Q function}
                \begin{align*}
                    & {A'}_\theta = f_\theta (\epsilon; S') \\
                    & \delta \leftarrow  R + \gamma (Q_{\phi}(S', {A'}_\theta) + \eta\mathcal{H}(\pi_{\theta}(\cdot| S'))) \\
                    & \quad \quad - Q_{\phi}(S, A_{\theta}) \\
                    & \phi  \leftarrow \phi - \alpha_Q \delta \; \nabla_{\phi} \; Q_{\phi}(S, a) \vert_{a=A_{\theta}} 
                \end{align*}
                % \vspace{-12pt}
                \STATE Update \emph{ Actor}
                \begin{align*}
                \theta \leftarrow \theta &+  \alpha_\pi \nabla_\theta (Q_{\phi}(S, A_{\theta}) + \eta\mathcal{H}{(\pi_{\theta}(\cdot| S))})
                \end{align*}
                \\
                \STATE $S \leftarrow S'$
        \ENDWHILE
        \ENDFOR
    \end{algorithmic}
    \end{spacing}
\end{algorithm}
\vspace{-0.75cm}
\end{minipage}
\end{wrapfigure}

We test the performance on AVG a simple 2D continuous control task termed \emph{Dot Reacher} and two MuJoCo tasks: \emph{Reacher-v4} and \emph{InvertedDoublePendulum-v4} from Farama Gymnasium \citep{towers_gymnasium_2023}. 
\paragraph{Dot Reacher} A dot object must reach a stationary target in a 2D plane by controlling its acceleration. The dot must also reach the target within a specific velocity threshold.
The observations include the position and velocity of the dot.
Acceleration applied to the dot in 2D, scaled from -1 to 1.
The dot starts at a random location, excluding the target region.
There are two variants - Easy and Hard.

We compare the performance of AVG against various established algorithms, including IAC, TD3, and SAC, using simple continuous control benchmarks.
First, we test 300 unique hyper-parameter configurations, each with 30 seeds. 
We then calculate the average undiscounted return for each run (i.e., area under the curve [AUC]).
Then, we average the AUC across all 30 seeds.
We plot the top 25 hyper-parameter configurations in Fig. \ref{fig:random_search_basic_envs} as a scatter plot, ranked in descending order from highest to lowest mean AUC.
Each plot point represents the mean AUC, and the thin lines denote the standard error.
Note that a point for a hyper-parameter configuration is plotted only if the configuration runs without diverging on all 30 random seeds.
These plots indicate which algorithm obtains the highest average episodic return and the robustness of the algorithms to the choice of hyper-parameters.
We select the hyper-parameter configuration with the highest average AUC as the best configuration and plot its learning curves in Fig. \ref{fig:lc_basic}.

\begin{figure}[ht]
    \centering
    \begin{subfigure}{.32\textwidth}
        \includegraphics[width=\columnwidth]{Figures/expt3/dot_reacher_hard_algo_comparison_best_seeds.png}
    \end{subfigure}
    \begin{subfigure}{.32\textwidth}
        \includegraphics[width=\columnwidth]{Figures/expt3/Reacher-v4_algo_comparison_best_seeds.png}
    \end{subfigure}
    \begin{subfigure}{.32\textwidth}
        \includegraphics[width=\columnwidth]{Figures/expt3/InvertedDoublePendulum-v4_algo_comparison_best_seeds.png}
    \end{subfigure}
    \caption{Learning curves of the best hyper-parameter configurations found via random search for each task variant.  Each solid curve is averaged over 30 independent runs. The shaded regions represent a 95\% confidence interval.}
    \label{fig:lc_basic}
    % \vspace{-15pt}
\end{figure}

Our experimental results show that AVG outperforms IAC, both with and without entropy, as well as the incremental variant of SAC (termed \emph{SAC-1}) on Reacher-v4 and InvertedPendulum-v4, both in terms of final performance and robustness to choice of hyper-parameters.
The incremental variant of TD3, termed \emph{TD3-1}, is very sensitive to the choice of random seed and hyper-parameters.
While it performs best on InvertedDoublePendulum-v4, it fails to solve the Dot Reacher task and produces only one good hyper-parameter configuration each for Reacher-v4 and InvertedDoublePendulum-v4.
Only this configuration runs without diverging on all 30 seeds.
